# Supplementary material for: To Add Is Machine, To Delete Is Human: Measuring and Mitigating Deletion Avoidance in LLM Code Editing
Source: arXiv:2607.28887 source file (2026-07-30)
Supplement: Supplementary file 1 [file Appendix.tex]

%% AAAI-27 Anonymous Submission -- supplementary material
%% Uses the same official AuthorKit27 template as the main paper.
\documentclass[letterpaper]{article} % DO NOT CHANGE THIS
\usepackage[submission]{aaai2027}  % DO NOT CHANGE THIS
\usepackage[hyphens]{url}  % DO NOT CHANGE THIS
\usepackage{graphicx} % DO NOT CHANGE THIS
\urlstyle{rm} % DO NOT CHANGE THIS
  % DO NOT CHANGE THIS
\usepackage{natbib}  % DO NOT CHANGE THIS AND DO NOT ADD ANY OPTIONS TO IT
\usepackage{caption} % DO NOT CHANGE THIS AND DO NOT ADD ANY OPTIONS TO IT

\usepackage{amsmath}
\usepackage{listings}
\usepackage{xcolor}
\usepackage{fvextra}
\usepackage{makecell}

\frenchspacing  % DO NOT CHANGE THIS
\usepackage{booktabs}
\pdfinfo{
/TemplateVersion (2027.1)
}

  \usepackage[most]{tcolorbox}
  \newtcolorbox{finding}{
    colback=black!6, colframe=black!6, boxrule=0pt, sharp corners,
    left=6pt, right=6pt, top=5pt, bottom=5pt,
    before skip=8pt, after skip=8pt}

\newcommand{\etal}[1]{et~al.}

% \textbf{}

% Provenance markers for the validity grid

%\newcommand{\rqfour}{RQ4: Your fourth research question?}
\newcommand{\showpagenumbers}{%
  \pagestyle{plain}%
  \thispagestyle{plain}%
}
\setcounter{secnumdepth}{2}

\title{Supplementary Material:\\{\Large Appendix}}
\author{}
\affiliations{}
\makeatletter
\gdef\showauthors@on{T}
\makeatother

\begin{document}

\maketitle
\showpagenumbers
\input{appendix-content}

\end{document}
